# Supplementary material for: Dual Structure-Aware Image Filterings for Semi-supervised Medical Image Segmentation
Source: arXiv:2312.07264 source file (2024-03-27)
Supplement: Supplementary file 1 [file tree_construction_suppl0.tex]

\begin{algorithm}
    \SetAlgoLined 
	\caption{Min-tree and Max-tree construction.}
        \label{alg:Min-MAX-tree-construction}
        \tcp{$\mathcal{R}$ : set of sorted pixels }
        \tcp{$N$ : total number of pixels}
        \tcp{$p, q, n, x$ : pixels}
        \tcp{$\mathcal{N}$ : neighbors}
        \tcp{$parent$ : image of parenthood}
        \tcp{$zpar$ : temporary parenthood}
        \tcp{$area$ : area of region}
	\KwIn{An image $f$.}
	\KwOut{Max-tree(Min-tree) of image $f$, areas of nodes.}

        \SetKwFunction{FROOT}{FIND\_ROOT}
        \SetKwProg{Fn}{Function}{:}{}
        \Fn{\FROOT{$x$}}{
            \Begin{ 
            \eIf{$zpar(x)=x$}{\textbf{return} $x$ }{$zpar(x) \leftarrow \FROOT{zpar(x)}$\;
            \textbf{return} $zpar(x)$
            }
            }
         }

        \SetKwFunction{UNION}{UNION\_FIND}
        \SetKwProg{Fn}{Function}{:}{}
        \Fn{\UNION{$\mathcal{R}$}}{
            \Begin{ 
            \For{ $p \in \mathcal{R}$}
            {$zpar(p) \leftarrow \text{undef}$\;
            $area(p) \leftarrow 0$ \;
            }
            
            \For{ $i = N-1:0$}
            {
            $p \leftarrow \mathcal{R}[i]$\;
            $parent(p) \leftarrow p$\;
            $zpar(p) \leftarrow p$ \;
            $area(p) \leftarrow 1$ \;
                \For{ $n \in \mathcal{N}(p) \cap zpar(n) \neq undef$}
                {
                    $r \leftarrow \FROOT{n}$\;             
                    \If{$r \neq p$}
                    {
                    $parent(r) \leftarrow p$ \;
                    $zpar(r) \leftarrow p$\;
                    $area(p) \leftarrow area(p)+area(r)$\;
                    }
                }
            
            }
            \textbf{return} $parent, area$
            }
      }

        \SetKwFunction{CANONIZE}{CANONIZE\_TREE}
        \SetKwProg{Fn}{Function}{:}{}
        \Fn{\CANONIZE{$f$, $\mathcal{R}$, $parent$}}{
            \Begin{ 
            \For{ $i = 0:N-1 $}{
            $p \leftarrow \mathcal{R}[i]$\;
            $q \leftarrow parent(p)$\; 
            \If{$f(parent(q)) = f(q)$}{$parent(p) \leftarrow parent(q)$ \;}
            
            }
            \textbf{return} $parent$
            }
        }

        % \SetKwFunction{MINMAX}{COMPUTE\_MIN\_MAX\_TREE}
        % \SetKwProg{Fn}{Function}{:}{}
        % \Fn{\MINMAX{$f$}}{
        % \Begin{
        % $\mathcal{R} \leftarrow \FuncSty{SORT\_MONOTONE}(f)$ \;
        % $parent,area \leftarrow$ \UNION{$\mathcal{R}$}\;
        % $parent \leftarrow$ \CANONIZE{f, $\mathcal{R}$, parent}\;
        % \textbf{return} $parent, area$
        % }
        % }
\end{algorithm}
