# Supplementary material for: Dual Structure-Aware Image Filterings for Semi-supervised Medical Image Segmentation
Source: arXiv:2312.07264 source file (2024-03-27)
Supplement: Supplementary file 2 [file min_max_suppl.tex]

\begin{algorithm}
    \SetAlgoLined 
	\caption{Min-tree and Max-tree construction.}
        \label{alg:min_max_suppl}
        \tcp{$\mathcal{R}$ : set of sorted pixels }
        \tcp{$N$ : total number of pixels}
        \tcp{$p, q$ : pixels}
        % \tcp{$\mathcal{N}$ : neighbors}
        \tcp{$parent$ : image of parenthood}
        % \tcp{$zpar$ : temporary parenthood}
        % \tcp{$area$ : area of region}
	\KwIn{An image $x$.}
	\KwOut{Max-tree(Min-tree) of image $x$, areas of nodes.}

        \SetKwFunction{CANONIZE}{CANONIZE\_TREE}
        \SetKwProg{Fn}{Function}{:}{}
        \Fn{\CANONIZE{$x$, $\mathcal{R}$, $parent$}}{
            \Begin{ 
            \For{ $i = 0:N-1 $}{
            $p \leftarrow \mathcal{R}[i]$\;
            $q \leftarrow parent(p)$\; 
            \If{$x(parent(q)) = x(q)$}{$parent(p) \leftarrow parent(q)$ \;}
            
            }
            \textbf{return} $parent$
            }
        }

        \SetKwFunction{MINMAX}{COMPUTE\_MIN\_MAX\_TREE}
        \SetKwProg{Fn}{Function}{:}{}
        \Fn{\MINMAX{$x$}}{
        \Begin{
        $\mathcal{R} \leftarrow \FuncSty{SORT\_MONOTONE}(x)$ \;
        $parent,area \leftarrow$ \UNION{$\mathcal{R}$}\;
        $parent \leftarrow$ \CANONIZE{x, $\mathcal{R}$, parent}\;
        \textbf{return} $parent, area$
        }
        }
\end{algorithm}
