# Supplementary material for: Dual Structure-Aware Image Filterings for Semi-supervised Medical Image Segmentation
Source: arXiv:2312.07264 source file (2024-03-27)
Supplement: Supplementary file 3 [file union_find_suppl.tex]

\begin{algorithm}
    \SetAlgoLined 
	\caption{Union find algorithm.}
        \label{alg:unifind_suppl}
        \tcp{$\mathcal{R}$ : set of sorted pixels }
        \tcp{$N$ : total number of pixels}
        \tcp{$p, q, v$ : pixels}
        \tcp{$\Omega$ : neighbors}
        \tcp{$parent$ : image of parenthood}
        \tcp{$zpar$ : temporary parenthood}
        \tcp{$area$ : area of region}
	\KwIn{An image $x$.}
	\KwOut{Max-tree(Min-tree) of image $x$, areas of nodes.}

        \SetKwFunction{FROOT}{FIND\_ROOT}
        \SetKwProg{Fn}{Function}{:}{}
        \Fn{\FROOT{$p$}}{
            \Begin{ 
            \eIf{$zpar(p)=p$}{\textbf{return} $p$ }{$zpar(p) \leftarrow \FROOT{zpar(p)}$\;
            \textbf{return} $zpar(p)$
            }
            }
         }

        \SetKwFunction{UNION}{UNION\_FIND}
        \SetKwProg{Fn}{Function}{:}{}
        \Fn{\UNION{$\mathcal{R}$}}{
            \Begin{ 
            \For{ $p \in \mathcal{R}$}
            {$zpar(p) \leftarrow \text{undef}$\;
            $area(p) \leftarrow 0$ \;
            }
            
            \For{ $i = N-1:0$}
            {
            $p \leftarrow \mathcal{R}[i]$\;
            $parent(p) \leftarrow p$\;
            $zpar(p) \leftarrow p$ \;
            $area(p) \leftarrow 1$ \;
                \For{ $q \in \Omega(p) \cap zpar(q) \neq undef$}
                {
                    $v \leftarrow \FROOT{q}$\;             
                    \If{$v \neq p$}
                    {
                    $parent(v) \leftarrow p$ \;
                    $zpar(v) \leftarrow p$\;
                    $area(p) \leftarrow area(p)+area(v)$\;
                    }
                }
            
            }
            \textbf{return} $parent, area$
            }
      }

\end{algorithm}
