# Supplementary material for: Dual Structure-Aware Image Filterings for Semi-supervised Medical Image Segmentation
Source: arXiv:2312.07264 source file (2024-03-27)
Supplement: Supplementary file 6 [file 10.tex]

\begin{table}[h]
\caption{Results after 10 steps of the $for$ loop from lines 13 to 24 in UNION\_FIND algorithm.}
\label{tab:10}
\centering

\begin{tabularx}{\linewidth}{|>{\centering\arraybackslash}X|>{\centering\arraybackslash}X|>{\centering\arraybackslash}X|>{\centering\arraybackslash}X|>{\centering\arraybackslash}X|>{\centering\arraybackslash}X|>{\centering\arraybackslash}X|}
%\toprule[1pt]
\hline
  { \footnotesize \cellcolor{gray!40} Step 10} &A  & B &C  &D  & E   \\
% \rowcolor{gray!40}
\hline
 \cellcolor{gray!40}P($\cdot$)   &E   &C  &D   & H  & F  \\
\hline

 \cellcolor{gray!40} ZPar($\cdot$)   &G  &H     &I    & H   & \textcolor{red}{I}       \\ 

\hline
\hline
  { \footnotesize \cellcolor{gray!40} Step 10} &F  &G  &H  &I  & J   \\
% \rowcolor{gray!40}
\hline
 \cellcolor{gray!40} P($\cdot$)   &G &H   & I    &\textcolor{red}{J}   & \textcolor{red}{J}  \\
\hline

 \cellcolor{gray!40}  ZPar($\cdot$)   &\textcolor{red}{J}  &\textcolor{red}{J}  & I    &\textcolor{red}{J}  &\textcolor{red}{J}       \\ 
\hline

\end{tabularx}

\end{table}
