# Supplementary material for: Dual Structure-Aware Image Filterings for Semi-supervised Medical Image Segmentation
Source: arXiv:2312.07264 source file (2024-03-27)
Supplement: Supplementary file 10 [file 5.tex]

\begin{table}[h]
\caption{Results after 5 steps of the $for$ loop from lines 13 to 24 in UNION\_FIND algorithm.}
\label{tab:5}
\centering

\begin{tabularx}{\linewidth}{|>{\centering\arraybackslash}X|>{\centering\arraybackslash}X|>{\centering\arraybackslash}X|>{\centering\arraybackslash}X|>{\centering\arraybackslash}X|>{\centering\arraybackslash}X|>{\centering\arraybackslash}X|}
%\toprule[1pt]
\hline
\cellcolor{gray!40} Step 5 &A  & B &C  &D  & E   \\
% \rowcolor{gray!40}
\hline
\cellcolor{gray!40}P($\cdot$)   &\textcolor{red}{E}   &C  &D   & D  & \textcolor{red}{E}  \\
\hline

\cellcolor{gray!40} ZPar($\cdot$)   &\textcolor{red}{E}  &C    &D   & D   &\textcolor{red}{E}        \\ 

\hline
\hline
\cellcolor{gray!40} Step 5 &F  &G  &H  &I  & J   \\
% \rowcolor{gray!40}
\hline
\cellcolor{gray!40} P($\cdot$)   &$undef$  &$undef$   &$undef$   & $undef$  & $undef$  \\
\hline

\cellcolor{gray!40}  ZPar($\cdot$)   &$undef$  &$undef$   &$undef$   & $undef$  & $undef$       \\ 
\hline

\end{tabularx}

\end{table}
