# Supplementary material for: Dual Structure-Aware Image Filterings for Semi-supervised Medical Image Segmentation
Source: arXiv:2312.07264 source file (2024-03-27)
Supplement: Supplementary file 14 [file 9.tex]

\begin{table}[h]
\caption{Results after 9 steps of the $for$ loop from lines 13 to 24 in UNION\_FIND algorithm.}
\label{tab:9}
\centering

\begin{tabularx}{\linewidth}{|>{\centering\arraybackslash}X|>{\centering\arraybackslash}X|>{\centering\arraybackslash}X|>{\centering\arraybackslash}X|>{\centering\arraybackslash}X|>{\centering\arraybackslash}X|>{\centering\arraybackslash}X|}
%\toprule[1pt]
\hline
\cellcolor{gray!40} Step 9 &A  & B &C  &D  & E   \\
% \rowcolor{gray!40}
\hline
\cellcolor{gray!40}P($\cdot$)   &E   &C  &D   & H  & F  \\
\hline

\cellcolor{gray!40} ZPar($\cdot$)   &G  &\textcolor{red}{H}     &\textcolor{red}{I}    & H   &G       \\ 

\hline
\hline
\cellcolor{gray!40} Step 9 &F  &G  &H  &I  & J   \\
% \rowcolor{gray!40}
\hline
\cellcolor{gray!40} P($\cdot$)   &G &H   & \textcolor{red}{I}    & \textcolor{red}{I}   & $undef$  \\
\hline

\cellcolor{gray!40}  ZPar($\cdot$)   &G  &\textcolor{red}{I}  & \textcolor{red}{I}     & \textcolor{red}{I}  & $undef$       \\ 
\hline

\end{tabularx}

\end{table}
