# Supplementary material for: Dual Structure-Aware Image Filterings for Semi-supervised Medical Image Segmentation
Source: arXiv:2312.07264 source file (2024-03-27)
Supplement: Supplementary file 15 [file bezier_ablation_suppl.tex]

\begin{table}[t]
  \centering
  \caption{Abaltion study on  B\'ezier curve using LA dataset~\citep{xiong2021global} under the setting of using 10\% labeled data}
  \label{tab:bezier_ablation_suppl}
  \setlength{\tabcolsep}{1mm}
    \resizebox{0.95\linewidth}{!}{
  \begin{tabular}{c|cccc}
    % \hline
    % \multicolumn{3}{c|}{Setting}  &\multicolumn{4}{c}{LA} \\
    \hline
    $z$  &Dice (\%) &JAC (\%) & 95HD  &ASD \\
    \hline
       CPS~\citep{chen2021semi}    &86.79   & 77.05  &14.19 &4.25 \\
        $\phi$   &89.77    & 81.51     & 6.79   &1.75  \\
    $\{0, 0.5\}$                                           &90.03   &81.94  &6.65     &1.77\\
     $\{0, 0.5, 0.75\}$                                   &90.33    &82.43      &6.53    &1.68 \\
     $\{0, 0.5, 0.75, 0.25\}$                             &89.64  & 81.30 &  7.25   & 1.81 \\
     $\{0, 0.5, 0.75, 0.25 , 0.875\}$                     &89.43   &80.96  &7.39    &1.87\\
      $\{0, 0.5, 0.75, 0.25 , 0.875,0.125\}$              &89.56   &81.16  &7.73    &1.93\\

    \hline
  \end{tabular}
  }
\end{table}
