# Supplementary material for: Dual Structure-Aware Image Filterings for Semi-supervised Medical Image Segmentation
Source: arXiv:2312.07264 source file (2024-03-27)
Supplement: Supplementary file 16 [file canonize.tex]

\begin{table}[t]
\caption{The process of CANONIZE\_TREE algorithm.}
\label{tab:canonize}
\centering

\begin{tabularx}{\linewidth}{|>{\centering\arraybackslash}X|>{\centering\arraybackslash}X|>{\centering\arraybackslash}X|>{\centering\arraybackslash}X|>{\centering\arraybackslash}X|>{\centering\arraybackslash}X|>{\centering\arraybackslash}X|}
%\toprule[1pt]
\hline
& \multicolumn{5}{c|}{$\xrightarrow{}$} \\
\hline
\cellcolor{gray!40}$p$ &J (4)  & I (4) &H (4)  &G (3)  & F (3)  \\
% \rowcolor{gray!40}
\hline
 { \cellcolor{gray!40} $q$} &$\phi$  &J (4)  &I (4)   &H (4)   & G (3) \\
\hline

\cellcolor{gray!40} $P(q)$   &$\phi$  &$\phi$   &J (4)   & J (4)  & J (4)      \\ 
\hline
\cellcolor{gray!40}Change   &$\phi$  &$\phi$   &{\footnotesize $P$(H)=J}   &{\footnotesize $P$(G)=J}   & $\phi$        \\ 
\hline
\hline
& \multicolumn{5}{c|}{$\xrightarrow{}$} \\
\hline
\cellcolor{gray!40} $p$        &E (2)  &D (2)  &C (2) &B (1) & A (1)  \\
% \rowcolor{gray!40}
\hline
 { \cellcolor{gray!40} $q$}    & F (3)   & H (4)  & D (2)  & C (2)   & E (2)  \\
\hline

\cellcolor{gray!40} $P(q)$     & G (3)   & J (4)   & J (4)   &  D (2) & G (3)      \\ 
\hline
\cellcolor{gray!40}Change      &{\footnotesize $P$(E)=G }   &{\footnotesize $P$(D)=J }    &$\phi$   &{\footnotesize $P$(B)=D }   & $\phi$        \\ 
\hline
\end{tabularx}

\end{table}
