# Supplementary material for: Dual Structure-Aware Image Filterings for Semi-supervised Medical Image Segmentation
Source: arXiv:2312.07264 source file (2024-03-27)
Supplement: Supplementary file 17 [file gamma_ablation_suppl.tex]

\begin{table}[t]
  \centering
  \caption{Abaltion study on  Gamma correction using LA dataset~\citep{xiong2021global} under the setting of using 10\% labeled data}
  \label{tab:gamma_ablation_suppl}
    \resizebox{0.95\linewidth}{!}{
  \begin{tabular}{c|cccc}
    \hline
    $[a,b]$  &Dice (\%) &JAC (\%) & 95HD  &ASD \\
    \hline
   CPS~\citep{chen2021semi}    &86.79   & 77.05  &14.19 &4.25 \\
      $[1,1]$   &88.46  &80.48    &10.19    &2.88     \\
     $[0.25,1.5]$   &89.19   &80.57     &8.30   &1.85 \\
    $[0.25,2]$      &90.06  & 81.98       & 7.38 &1.83 \\
    $[0.25,4]$      &89.46    &81.00     &7.65    &1.78 \\
     $[0.5,1.5]$   &90.33    &82.43      &6.53    &1.68 \\
   $[0.5,2]$     &90.11     & 82.08   &6.61   &1.69 \\
  $ [0.5,3] $    &89.86    &81.66      & 6.77    & 1.73\\
    $[0.5,4]$   & 89.56    &81.15     &7.17    & 1.70\\

    \hline
  \end{tabular}
  }
\end{table}
