# Supplementary material for: Dual Structure-Aware Image Filterings for Semi-supervised Medical Image Segmentation
Source: arXiv:2312.07264 source file (2024-03-27)
Supplement: Supplementary file 18 [file increase0.tex]

\begin{table}[t]
\caption{Employing monotonically increasing contrast changes to adjust the image contrast.}
\label{tab:increase0}
\centering

\begin{tabular}{|c|c|c|c|c|}
%\toprule[1pt]
\hline
2   & 2  &4   &1 & 3 \\
\hline
1  &4  &3 &2  &4   \\
\hline
 \multicolumn{5}{c}{$\Downarrow$} \\
\hline
4   & 4  &8   &2 & 6 \\
\hline
2  &8  &6 &4  &8   \\
\hline
\end{tabular}

\end{table}
