# Supplementary material for: Dual Structure-Aware Image Filterings for Semi-supervised Medical Image Segmentation
Source: arXiv:2312.07264 source file (2024-03-27)
Supplement: Supplementary file 19 [file increase1.tex]

\begin{table}[b]
\caption{Increasing order of pixels after employing monotonically increasing contrast changes to adjust the image contrast.}
\label{tab:increase1}
\centering

\begin{tabular}{|c|c|c|c|c|}
%\toprule[1pt]
\hline
2 (C)  & 2 (D) &4 (H)  &1 (A) & 3 (F)  \\
\hline
1 (B) &4 (I) &3 (G) &2 (E) &4 (J)  \\
\hline
 \multicolumn{5}{c}{$\Downarrow$} \\
\hline
4 (C)  & 4 (D) &8 (H)  &2 (A) & 6 (F)  \\
\hline
2 (B) &8 (I) &6 (G) &4 (E) &8 (J)  \\
\hline
 
\end{tabular}

\end{table}
